# Supplementary material for: Learning Visuo-Motor Behaviours for Robot Locomotion Over Difficult Terrain
Source: arXiv:2303.01634 source file (2023-03-02)
Supplement: Supplementary file 1 [file Ch7Appendix.tex]

\appendix[Example I]{Example I without Detailed Explanations} 
\label{app:A}

\appendix[Example II]{Example II with Detailed Explanations}
\label{app:B}
