# Supplementary material for: Learning Visuo-Motor Behaviours for Robot Locomotion Over Difficult Terrain
Source: arXiv:2303.01634 source file (2023-03-02)
Supplement: Supplementary file 2 [file Appendix.tex]

%%%%%%%%%%%%%%%%%%%%%%
%\appendix[Appendix A: Example I]{Appendix A: Example I} 
\appendix[Example I]{Example I without Detailed Explanations} 
\label{app:A}

This is the first appendix. 

%====================
\section{Problem Formulation}

The problem can be described using the following state space model
\begin{equation}
\dot{x(t)} = Ax(t) + Bu(t) + Gw(t)
\label{eqn:statespacemodel}
\end{equation}
where $x$ is the system state. 

%===================
\section{Solving the Problem}
To solve this problem, a new method is proposed. .....

The simulation results are shown in Table \ref{tab:sim}. 

\begin{table}
 \begin{center}
  \caption{Simulation results.}
  \label{tab:sim}
  \begin{tabular}{cc}
   \hline
    Time $t$ & Output $y(t)$\\
   \hline
    1 & 10 \\
    2 & 12\\
    3 & 15\\
   \hline
  \end{tabular}
 \end{center}
\end{table}

%%%%%%%%%%%%%%%%%%%%%%%%%%%%%%%%%%%%%%%%
\appendix[Example II]{Example II with Detailed Explanations}
\label{app:B}

This is the 2nd appendix. 

%====================
\section{System Output Model}

The model to describe the system output dynamics is given by
\begin{equation}
 y(t) = Cx(t) + Hv(t)
\label{eqn:output}
\end{equation}

%=======================
\section{Simulation for System Output}

Simulation results of the system dynamic model are given Table \ref{tab:output}.

\begin{table}
 \begin{center}
  \caption{Simulation results of the system output model.}
  \label{tab:output}
  \begin{tabular}{cc}
   \hline
    Time $t$ & State $x(t)$\\
   \hline
    1 & 10 \\
    2 & 12\\
    3 & 15\\
   \hline
  \end{tabular}
 \end{center}
\end{table}
